# Supplementary material for: Boosting Diffusion Guidance via Learning Degradation-Aware Models for Blind Super Resolution
Source: arXiv:2501.08819 source file (2025-01-23)
Supplement: Supplementary file 1 [file supp_main.tex]

% WACV 2025 Paper Template
% based on the WACV 2024 template, which is
% based on the CVPR 2023 template (https://media.icml.cc/Conferences/CVPR2023/cvpr2023-author_kit-v1_1-1.zip) with 2-track changes from the WACV 2023 template (https://github.com/wacv-pcs/WACV-2023-Author-Kit)
% based on the CVPR template provided by Ming-Ming Cheng (https://github.com/MCG-NKU/CVPR_Template)
% modified and extended by Stefan Roth (stefan.roth@NOSPAMtu-darmstadt.de)

\documentclass[10pt,twocolumn,letterpaper]{article}

%%%%%%%%% PAPER TYPE  - PLEASE UPDATE FOR FINAL VERSION
% \usepackage[review,algorithms]{wacv}      % To produce the REVIEW version for the algorithms track
%\usepackage[review,applications]{wacv}      % To produce the REVIEW version for the applications track
\usepackage{wacv}              % To produce the CAMERA-READY version
%\usepackage[pagenumbers]{wacv} % To force page numbers, e.g. for an arXiv version

% Include other packages here, before hyperref.
\usepackage{graphicx}
\usepackage{amsmath}
\usepackage{amssymb}
\usepackage{booktabs}
\usepackage{multirow}
\usepackage[table,xcdraw]{xcolor}
% Beamer presentation requires \usepackage{colortbl} instead of \usepackage[table,xcdraw]{xcolor}
\usepackage[normalem]{ulem}
\useunder{\uline}{\ul}{}
\usepackage{adjustbox}

% It is strongly recommended to use hyperref, especially for the review version.
% hyperref with option pagebackref eases the reviewers' job.
% Please disable hyperref *only* if you encounter grave issues, e.g. with the
% file validation for the camera-ready version.
%
% If you comment hyperref and then uncomment it, you should delete
% ReviewTempalte.aux before re-running LaTeX.
% (Or just hit 'q' on the first LaTeX run, let it finish, and you
%  should be clear).
\usepackage[pagebackref,breaklinks,colorlinks]{hyperref}

\newcommand{\heading}[1]{\vspace{1mm}\noindent\textbf{#1}}
% Support for easy cross-referencing
\usepackage[capitalize]{cleveref}
\crefname{section}{Sec.}{Secs.}
\Crefname{section}{Section}{Sections}
\Crefname{table}{Table}{Tables}
\crefname{table}{Tab.}{Tabs.}

%%%%%%%%% PAPER ID  - PLEASE UPDATE
 % *** Enter the WACV Paper ID here

\begin{document}

%%%%%%%%% TITLE - PLEASE UPDATE
\title{Boosting Diffusion Guidance via Learning Degradation-Aware Models \\ for Blind Super Resolution \\
 \large [Supplementary Material]}

% \author{Shao-Hao Lu\inst{1} \and
% Ren Wang\inst{2} \and
% Ching-Chun Huang\inst{1} \and
% Wei-Chen Chiu\inst{1}}

% \institute{National Yang Ming Chiao Tung University \and MediaTek Inc. \\
% \email{\{shlu2240.cs11, chingchun, walon\}@nycu.edu.tw, ren.wang@mediatek.com}
% }
\author{Shao-Hao Lu$^{1}$ \qquad Ren Wang$^{2}$ \qquad Ching-Chun Huang $^{1}$ \qquad Wei-Chen Chiu$^{1}$ 
\\
{\small\tt $^{1}$National Yang Ming Chiao Tung University \qquad $^{2}$MediaTek Inc.}
\\
{\small\tt \{shlu2240.cs11, chingchun, walon\}@nycu.edu.tw \qquad ren.wang@mediatek.com}}

% \author{Shao-Hao Lu$^{\dagger}$ \qquad Ren Wang$^{\ddagger}$ \qquad Ching-Chun Huang $^{\dagger}$ \qquad Wei-Chen Chiu$^{\dagger}$ 
% \\
% {\small\tt $^{\dagger}$National Yang Ming Chiao Tung University, Taiwan \qquad $^{\ddagger}$MediaTek Inc.}}

\maketitle

\definecolor{gold}{RGB}{0, 0, 0}
\newcommand{\ren}[1]{{\color{gold}#1}\normalfont}
\newcommand{\walon}[1]{{\color{red}#1}\normalfont}

Here, we provide
1) the details of training data preparation,
2) methodology of the explicit kernel estimator used in our ablation study for both the \emph{explicit} and \emph{combine} experiments, and
3) more qualitative results.

\section{Training Data Preparation}
To train our degradation and restoration models, we need to generate LR-HR paired data. For the DIV2K dataset with unknown degradation, the LR-HR paired images have been provided, and we just randomly crop HR patches of resolution $256 \times 256$ and their corresponding LR patches of resolution $64 \times 64$ during training.

For the CelebA-HQ dataset, which only consists of HR images, we generate LR images by performing convolution with random anti-isotropic Gaussian kernels, where the stride is equal to the degradation scale.
Following Wang \etal \cite{wang2021unsupervised}, we diversify these kernels by sampling some additional parameters. Specifically, the filter size is sampled from the odd numbers in the range of $[7, 21]$. The weights are determined by two eigenvalues $\lambda_1$ and $\lambda_2$ of a covariance matrix, both of which are sampled from a uniform distribution $\mathcal{U}(0.2, 4)$. We also apply rotation to these kernels with an angle $\theta \sim \mathcal{U}(0, \pi)$.

\section{Explicit Kernel Estimator}
Both of our \emph{explicit} and \emph{combine} approaches involve integrating an explicit kernel estimator into DDNM \cite{wang2022zero}. Given a degraded image \ren{$\mathbf{y}$}, the estimator \(\cal{E}\) predicts the corresponding degradation kernel. Following the architecture proposed by Lian \etal \cite{lian2023kernel}, we train the estimator using the ground truth kernel as supervision. The training objective aims to minimize the \(\mathcal{L}_1\) loss between the estimated kernel and the ground truth 
 kernel \ren{$\mathbf{k}$ as}
\begin{equation}
\mathcal{L}_k = \| \mathbf{k} - \mathcal{E}(\mathbf{y};\theta_{e}) \|_{1} \ren{.}
\end{equation}

After obtaining the predicted kernel, we turn the convolution with this kernel into a matrix multiplication with a matrix \ren{$\mathbf{A}$}. Furthermore, we can compute its pseudo-inverse \ren{$\mathbf{A}^\dagger$} using SVD, and directly plug \ren{$\mathbf{A}$} and \ren{$\mathbf{A}^\dagger$} into DDNM. However, this explicit kernel estimator assumes the degradation is a convolution with kernel, which might lead to over-simplification.
Therefore, our \emph{implicit} method shows better performance than \emph{explicit} and \emph{combine} methods in the ablation study.

Note that we do not have ground-truth kernels for the DIV2K dataset with unknown degradation, which are necessary to train the estimator $\mathcal{E}$. As a result, we adopt the pipeline used for generating training data to sample kernels, and use them to not only generate LR-HR pairs but also train the estimator $\mathcal{E}$.

\section{More Qualitative Results}
We provide more qualitative results on the \emph{ImageNet-Val} and \emph{CelebA-Val} datasets in Figs.~\ref{fig:imagenet_x4}--\ref{fig:celeba_x8}.

\begin{figure*}
    \centering
    \includegraphics[width=1\linewidth]{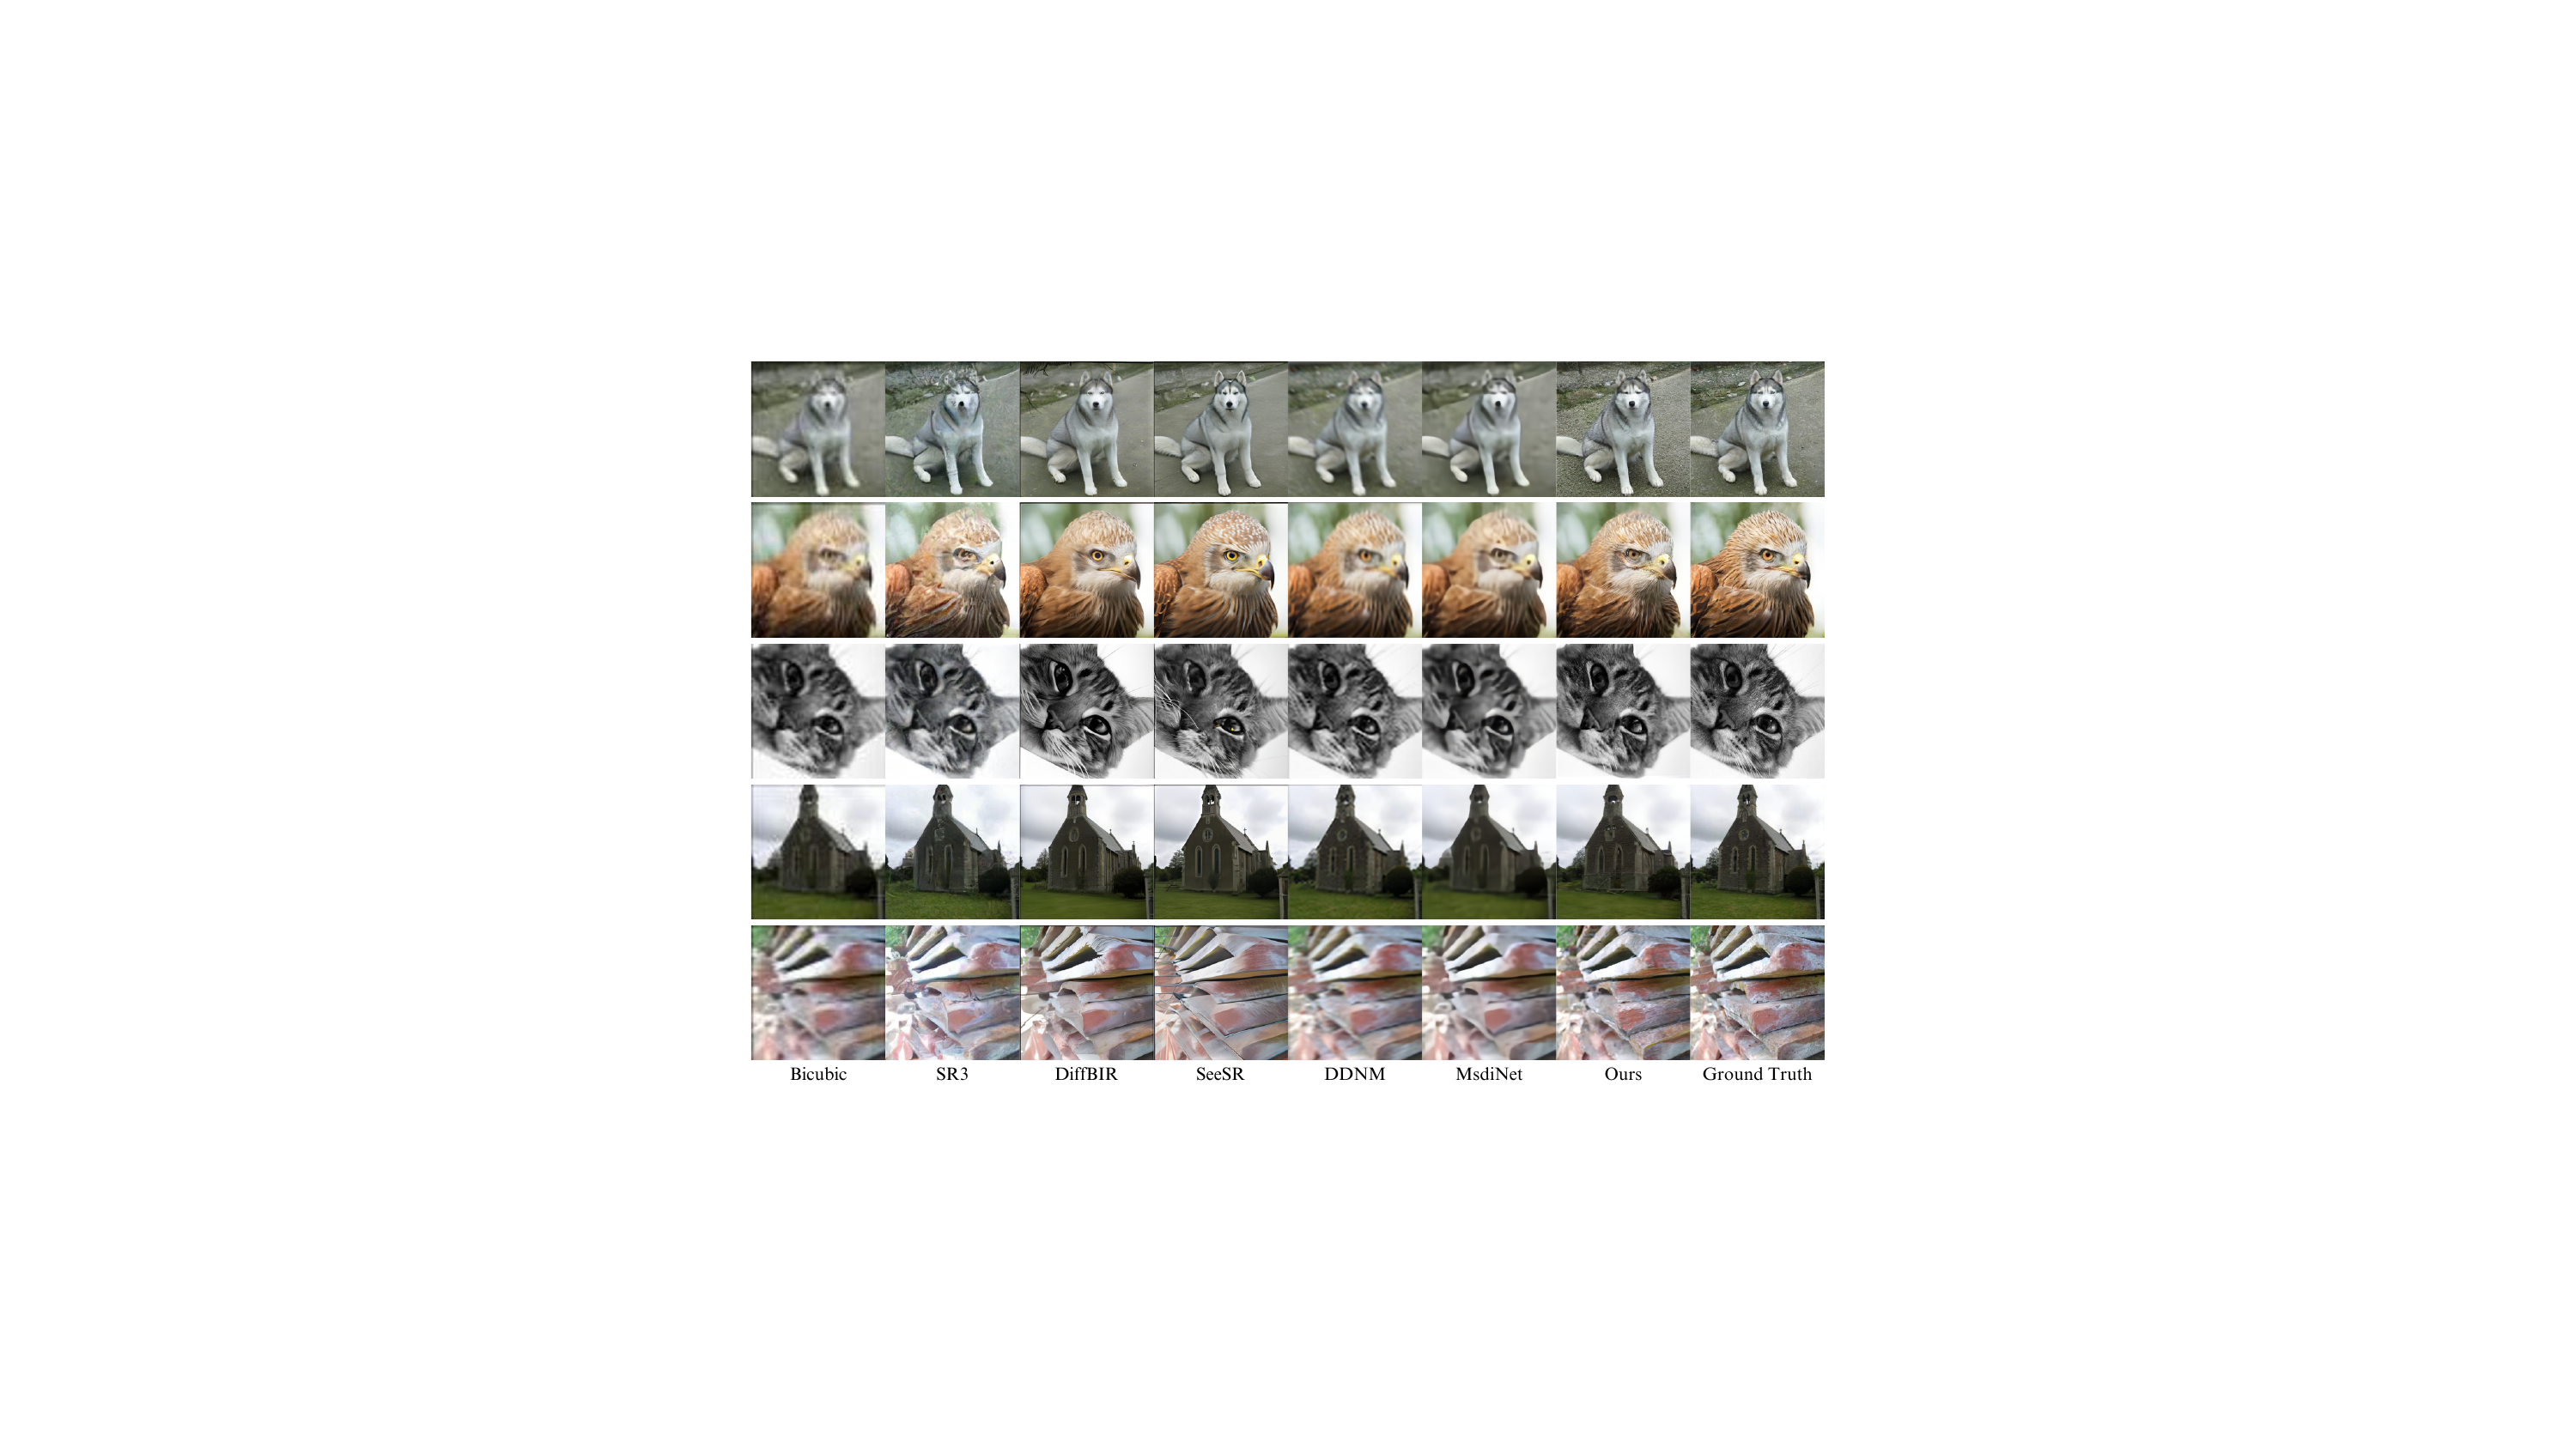}
    \caption{\heading{Qualitative comparison of $\bf{4 \times}$ upsampling on \emph{ImageNet-Val}.}}
    \label{fig:imagenet_x4}
\end{figure*}

\begin{figure*}
    \centering
    \includegraphics[width=1\linewidth]{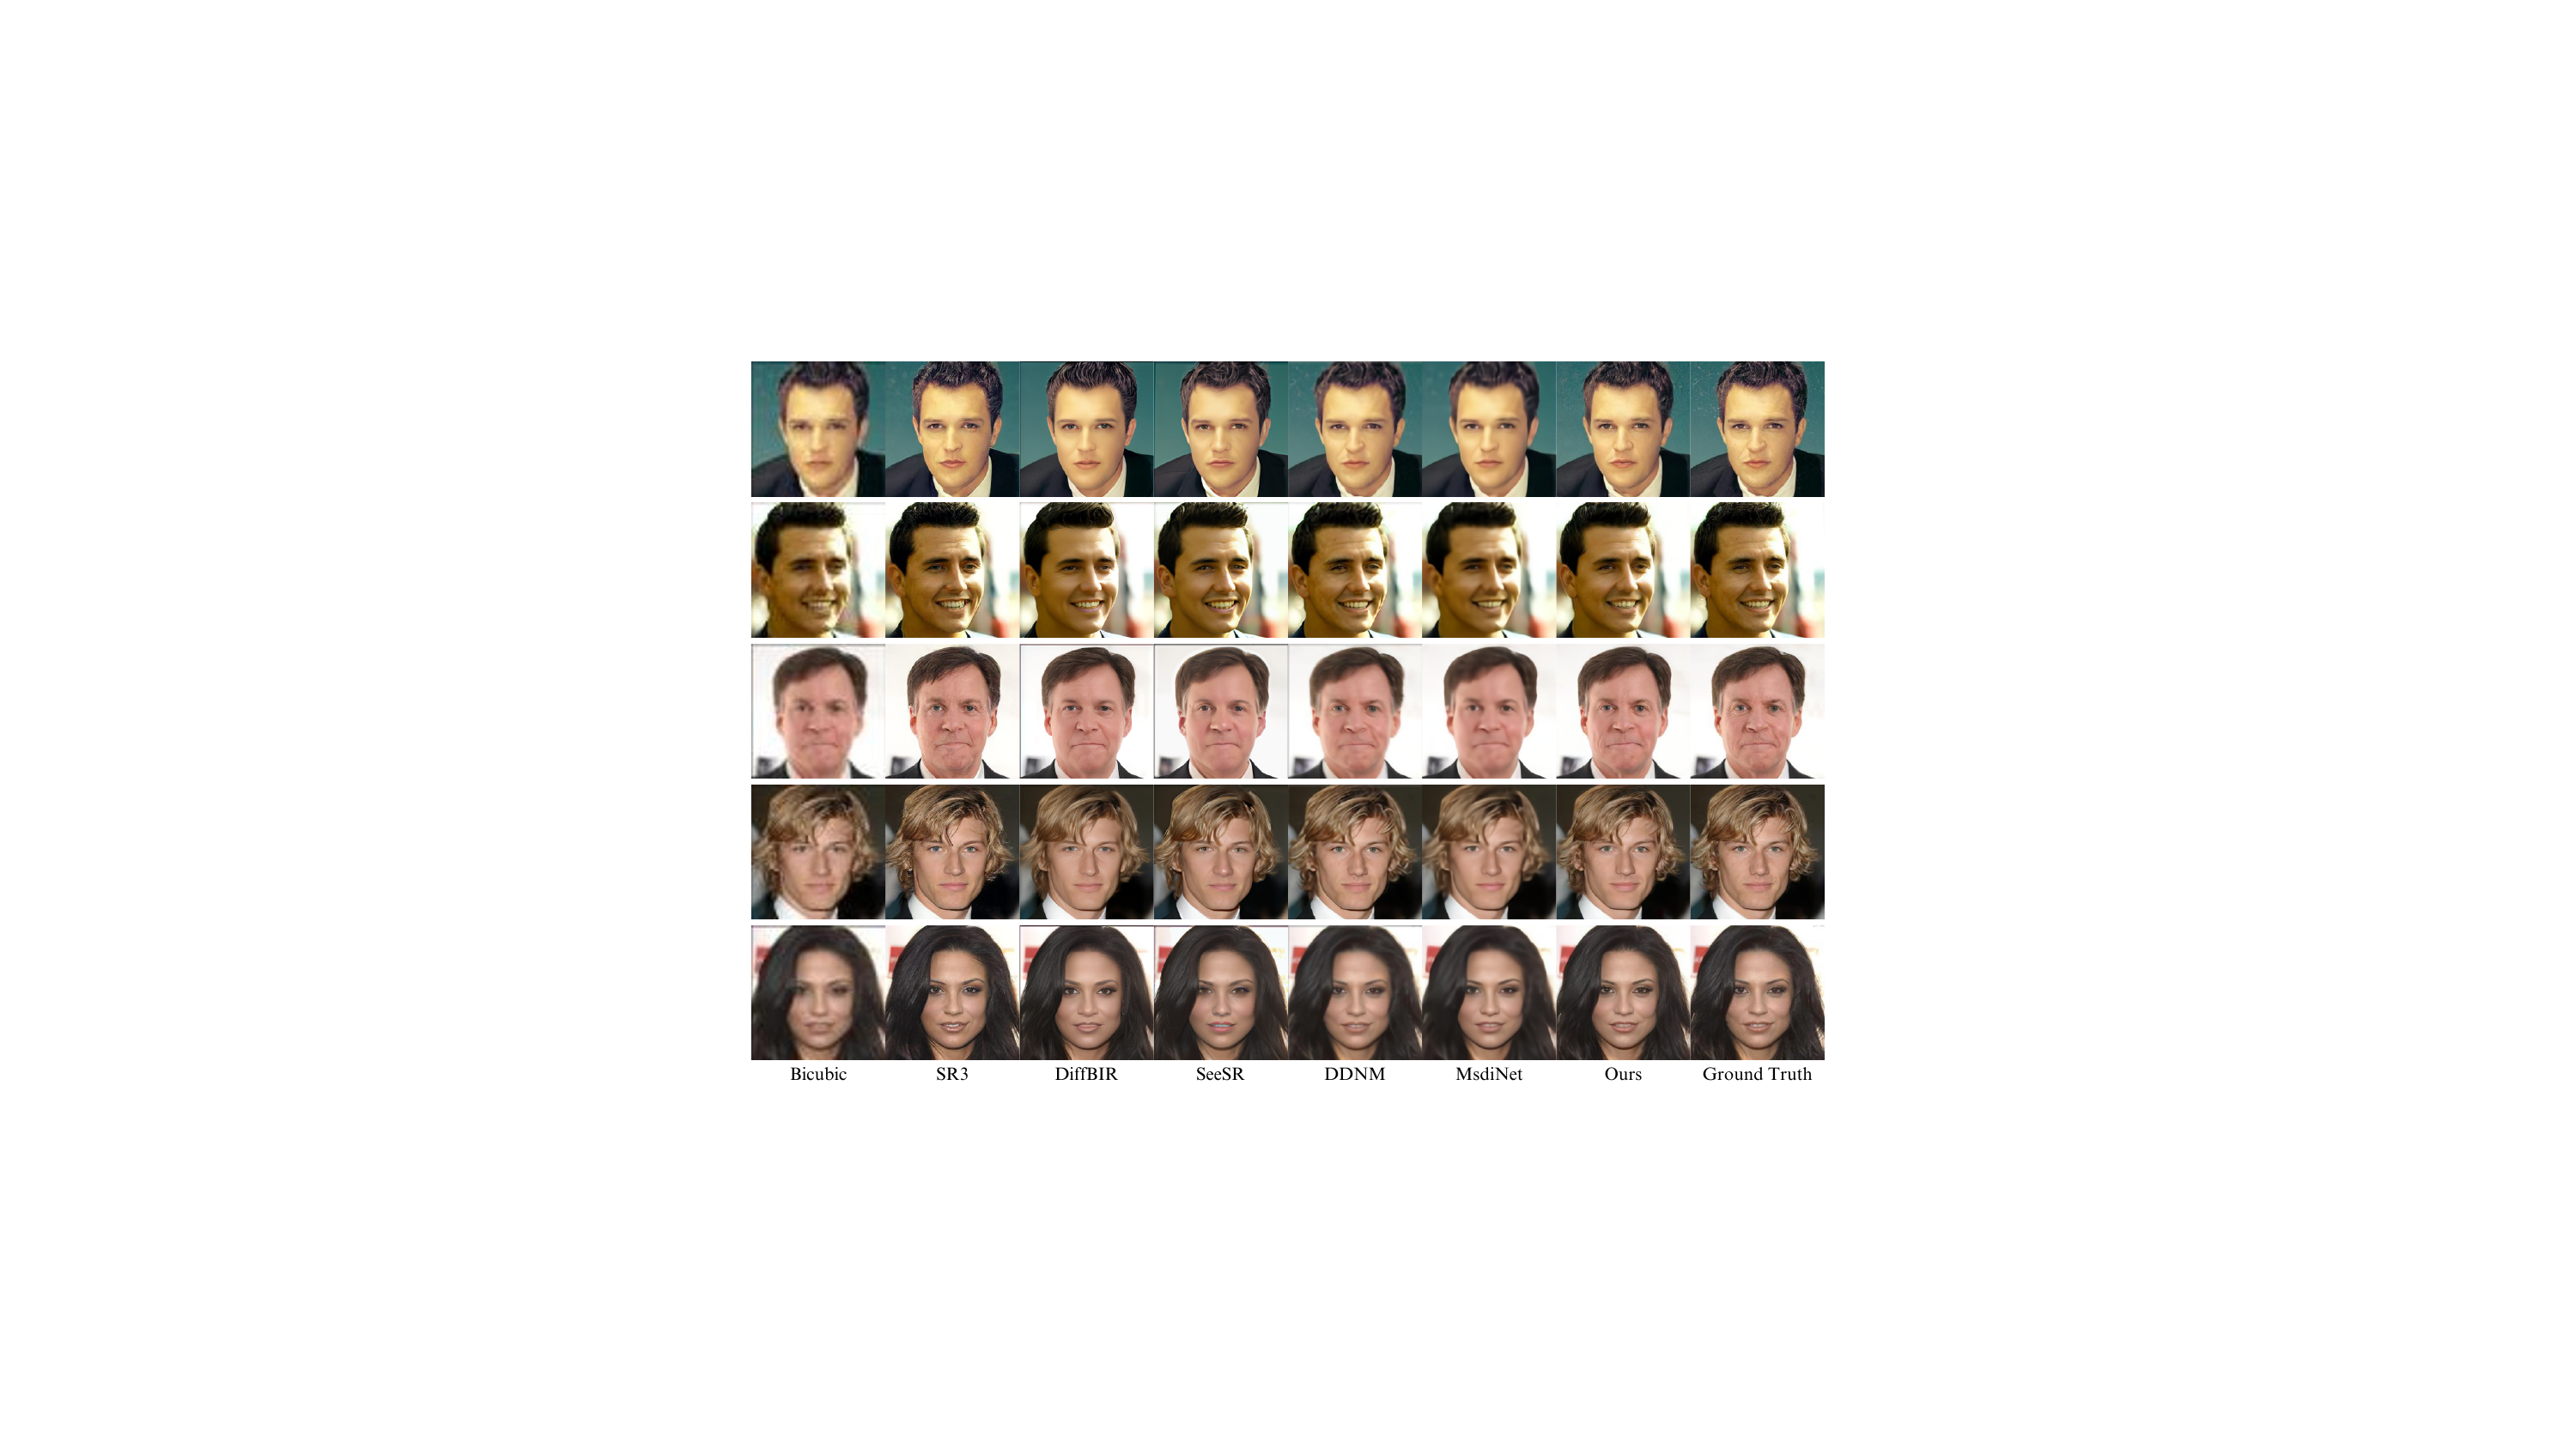}
    \caption{\heading{Qualitative comparison of $\bf{4 \times}$ upsampling on \emph{CelebA-Val}.}}
    \vspace{-0.3cm}
    \label{fig:celeba_x4}
\end{figure*}

\begin{figure*}
    \centering
    \includegraphics[width=1\linewidth]{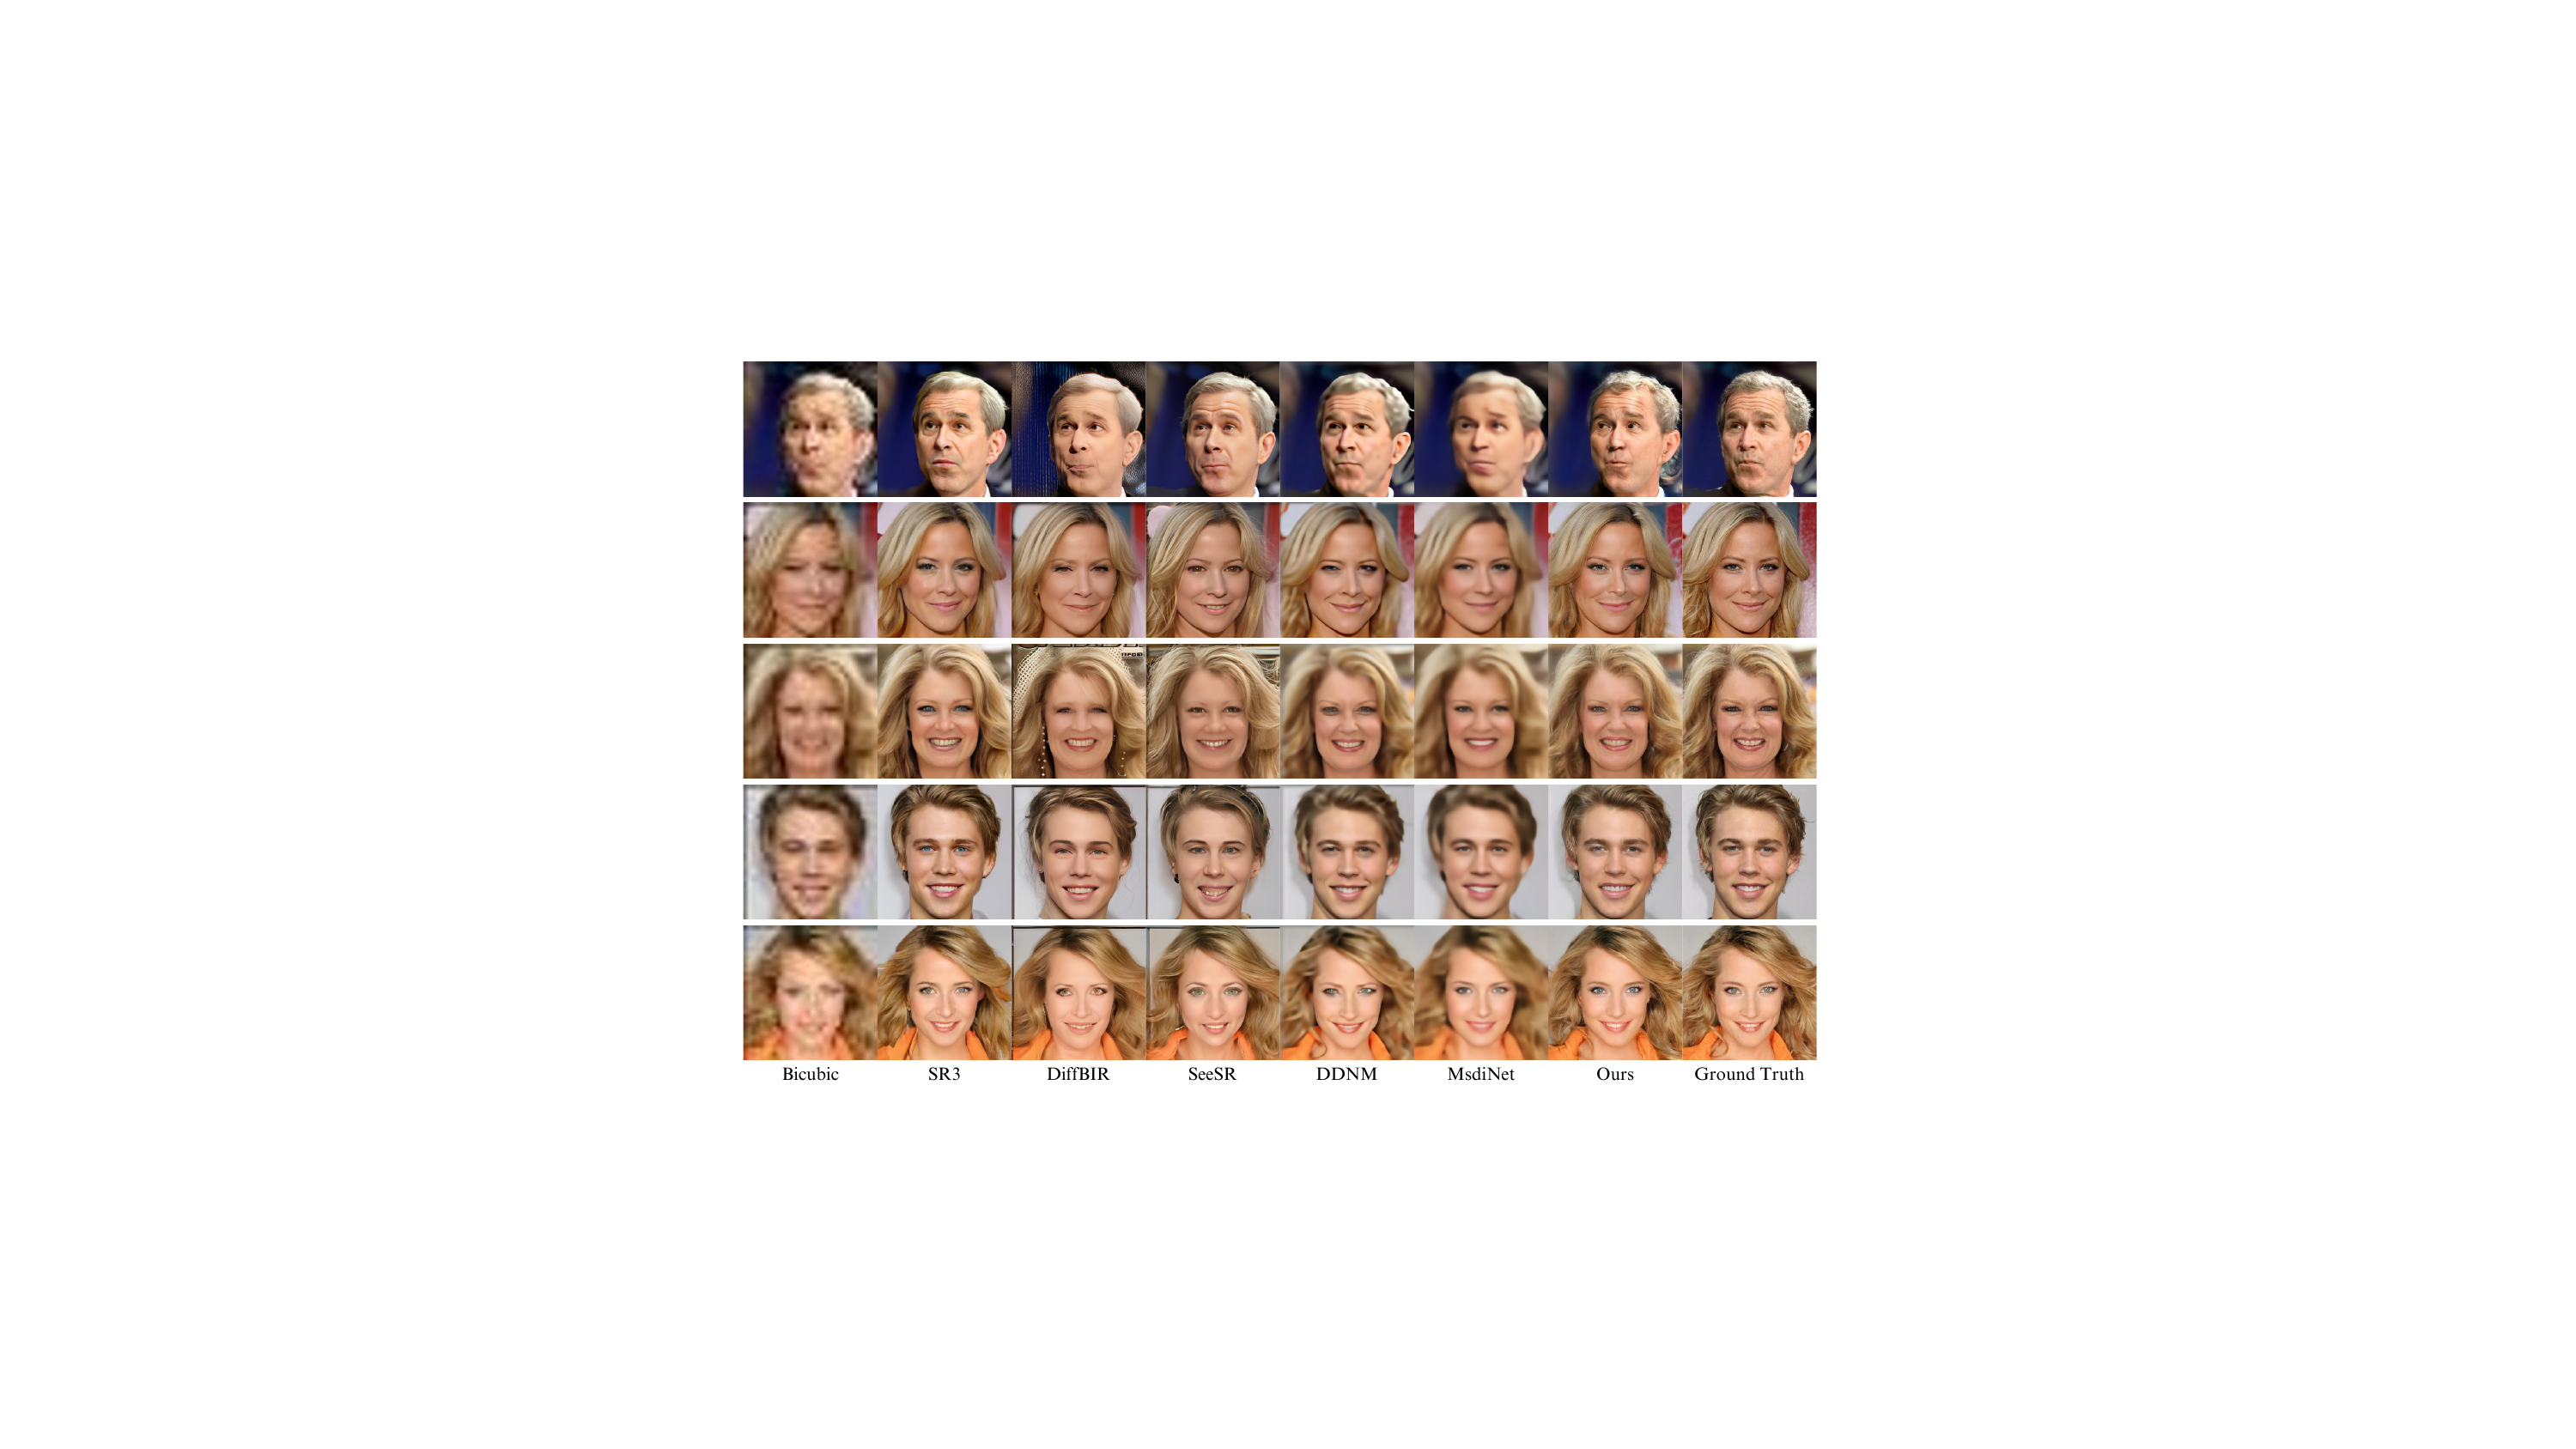}
    \caption{\heading{Qualitative comparison of $\bf{8 \times}$ upsampling on \emph{CelebA-Val}.}}
    \label{fig:celeba_x8}
\end{figure*}

%%%%%%%%% REFERENCES
{\small
\bibliographystyle{ieee_fullname}
\bibliography{egbib}
}

\end{document}
